# Supplementary material for: Towards Dynamic Simulations of Materials on Quantum Computers
Source: arXiv:2004.04836 ancillary file (2020-04-09)
Supplement: Supplementary file 1 [file SupplementalMaterial.pdf]

## Supplemental Material

### Towards Dynamic Simulations of Materials on Quantum Computers

Lindsay Bassman,<sup>1\*</sup> Kuang Liu,<sup>1</sup> Aravind Krishnamoorthy,<sup>1</sup> Thomas Linker,<sup>1</sup> Yifan Geng,<sup>1</sup>

Daniel Shebib,<sup>1</sup> Shogo Fukushima,<sup>2</sup> Fuyuki Shimojo,<sup>2</sup> Rajiv K. Kalia,<sup>1</sup> Aiichiro Nakano,<sup>1</sup> and

Priya Vashishta<sup>1</sup>

<sup>1</sup> *Collaboratory for Advanced Computing and Simulations, University of Southern California, Los Angeles, CA 90089-0242, United States of America*

<sup>2</sup> *Department of Physics, Kumamoto University, Kumamoto 860-8555, Japan*

\*Correspondence to: bassman@usc.edu

### Python Notebooks for Dynamic Simulations on IBM and Rigetti Quantum Computers

Python notebooks entitled ‘QiskitDemo.ipynb’ and ‘PyQuilDemo.ipynb’ can be found at [https://github.com/lebassman/TFIM\\_Trotter\\_Simulations](https://github.com/lebassman/TFIM_Trotter_Simulations). They demonstrate how to perform dynamic quantum simulations on the IBM and Rigetti quantum computers, respectively. Full code and step-by-step tutorials for creating quantum circuits, connecting to the quantum computer, running the simulations, and post-processing the raw data are included in the notebooks.

### First-Principles Calculation of Exchange Interaction

First principles calculations based on spin-polarized density functional theory (DFT) are used to compute the exchange interaction term  $J_z$ . The system used is a monolayer of ReSe<sub>2</sub> and includes 108 atoms, corresponding to  $6 \times 6 \times 1$  unit cells in a box of dimensions  $19.728 \times 19.728 \times 16.2 \text{ \AA}^3$  with periodic boundary conditions applied in all directions (see Fig. S1). This box includes a vacuum of  $12 \text{ \AA}$  along the perpendicular direction to avoid spurious interactions between neighboring images of the monolayer. The electronic states are calculated using the projector augmented-wave (PAW) method [1,2]. Projector functions are generated for 5d, 6s, and 6p states of rhenium (Re) and for the 4s, 4p, and 4d states of selenium (Se). The generalized gradient approximation (GGA) is used for the exchange-correlation energy [3]. To more accurately assess the effect of on-site Coulomb repulsion among the localized electrons in the partially filled  $d$  subshells, the DFT+U method [4] was employed with the parameters  $U_{\text{eff}} =$

1.5 eV [5] for Re 5d electrons. The van der Waals interaction between atoms is described with the DFT-D approach [6]. The momentum-space formalism was utilized, where the plane-wave cutoff energies are 30 and 250 Ry for the electronic pseudo-wave functions and pseudo-charge density, respectively. The  $\Gamma$  point is used for Brillouin zone sampling for electronic-structure calculations. We use our own scalable parallel quantum molecular dynamics (QMD) simulation software for the first principles calculation [7,8].

The local magnetic moments were obtained as  $|M_s| = 0.68$  and  $0.048 \mu_B/\text{atom}$  for Re and Se, respectively. The exchange interaction parameter  $J_z$  is obtained according to the equation

$$J_z = \frac{E_{\text{AFM}} - E_{\text{FM}}}{4\mu_{\text{uc}}^2}, \quad (\text{S1})$$

where  $\mu_{\text{uc}}$  is a net magnetic moment per unit cell,  $E_{\text{FM}}$  and  $E_{\text{AFM}}$  are the energy per unit cell in ferromagnetic and anti-ferromagnetic alignment, respectively [9]. Equation S1 gives a value of  $J_z = 0.01183898$  eV for this material. Note that the unit cells for the ferromagnetic system and antiferromagnetic system are different, as shown in Fig. S1, and also differ from the usual smallest unit cell of  $\text{ReSe}_2$  when ignoring spin.

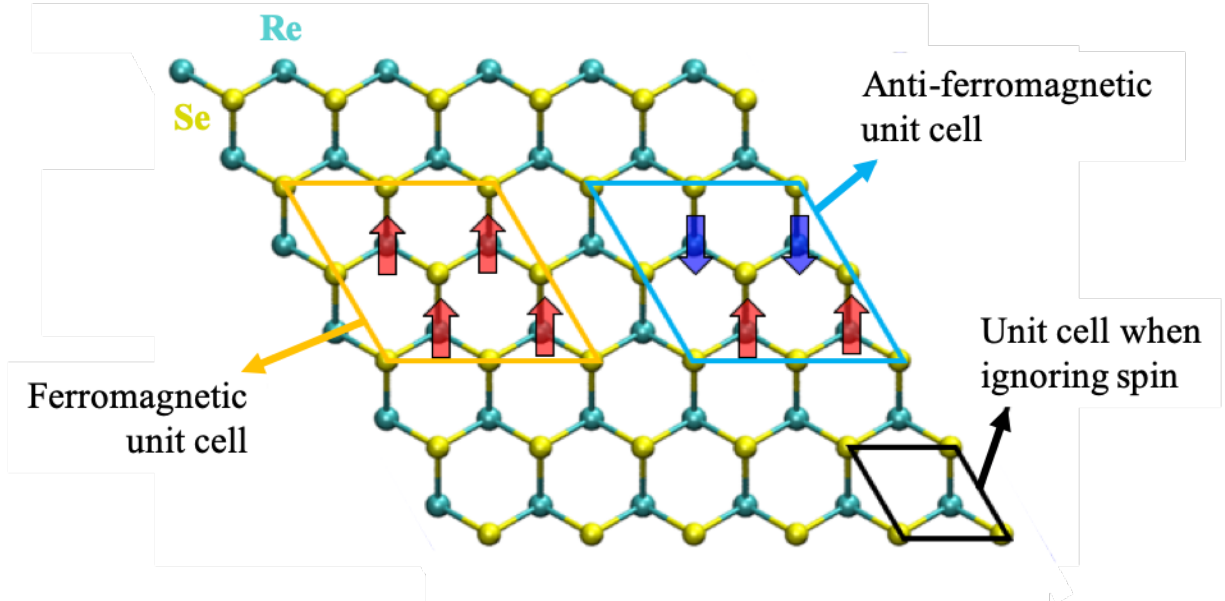

FIG. S1. Schematic describing the calculation of the exchange interaction term  $J_z$  between unpaired electron spins in neighboring Re atoms. Re atoms are depicted by cyan spheres, while Se atoms are depicted by yellow spheres. The red block arrows indicate the unpaired electron of the Re atom is spin-up, while the blue block arrows denote spin-down.

## Emergent Transverse Magnetic Field from $E''$ Phonon Activation

Specific phonon modes of 2D materials can be controlled through ultra-fast terahertz excitation of phonons by controlled laser pulses [10]. Spin orbit coupling (SOC) interactions of electrons in the material can then be coupled to the active phonon mode as a result of an effective gauge field induced by the active phonon momentum [11]. To illustrate this effect in MoSe<sub>2</sub> (top view shown in Fig. S2a), we have calculated the Zeeman splitting of spins states at the conduction band minimum (CBM) in the K valley as a result of a displacement of 0.1 Å along the E'' mode as shown in Fig. S2, b and c. We found a 3 meV splitting of the two spin states at the CBM as a result of the displacement. This phonon-induced field can be modeled as an effective transverse magnetic field with magnitude  $B(t) = \varepsilon_{ph} \sin(\omega_{ph}t)$ , where  $\varepsilon_{ph}$  implicitly depends on the magnitude of the displacement along the E'' mode and  $\omega_{ph}$  is the experimentally measured phonon frequency [11]. The strength of  $\varepsilon_{ph}$  or displacement of the atoms depends on the fluence of the laser in a terahertz excitation experiment.

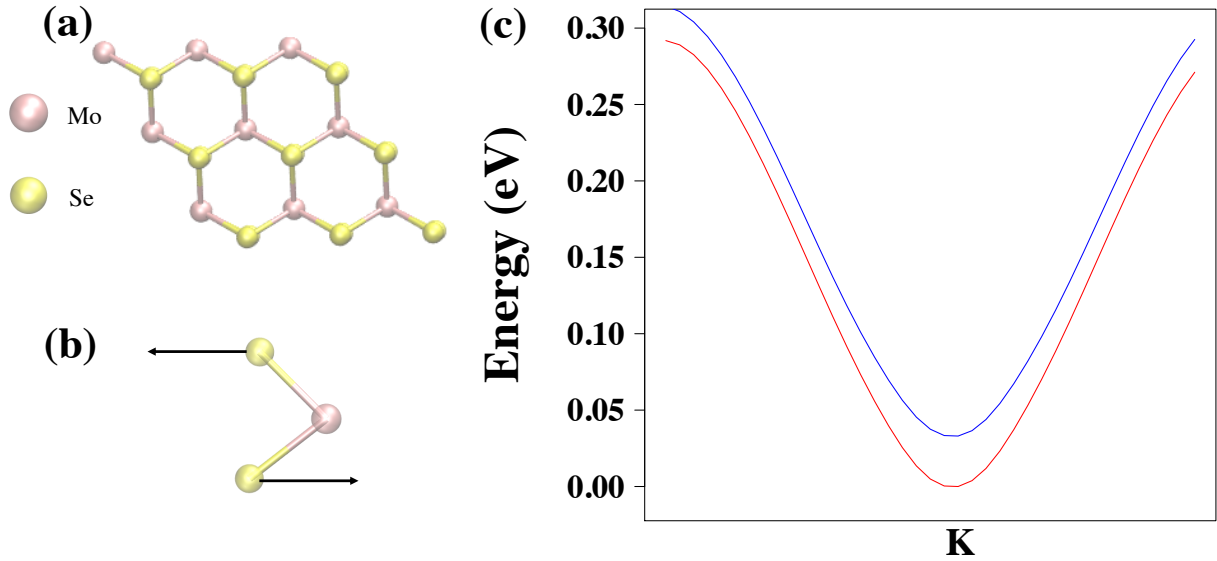

FIG. S2. K-valley splitting. (a) top view of MoSe<sub>2</sub>. (b) side view of MoSe<sub>2</sub> with displacement indicated along the E'' phonon mode. (c) the resulting splitting of the spin states in the K valley at the conduction band minimum due to a displacement along E'' phonon mode of 0.1 Å.

To calculate the splitting of the K-valley in MoSe<sub>2</sub> we used the Vienna Ab-Initio Software Package (VASP) [12]. Electronic states were calculated with a plane-wave basis with an energy cutoff of 500 eV and the Project Augmented Wave (PAW) method [1] with SOC. To approximate the exchange-correlation functional, we used a Perdew-Burke-Ernzerhof type generalized gradient approximation [3]. We performed the calculation on a MoSe<sub>2</sub> unit cell with a lattice constant of

3.289 Å. 16 Å of vacuum were added along the [0 0 1] direction to simulate a MoSe<sub>2</sub> monolayer. The Brillouin zone was sampled by Monkhorst-Pack sampling of a  $15 \times 15 \times 3$  k-point grid.

### Sample Quantum Circuit Diagram

A quantum circuit diagram for the simulation of one time-step of evolution for a three-qubit system under Hamiltonian (1) in the main text is shown in Fig. S3. The top three horizontal lines in the diagram represent the three qubits, while the bottom line represents the three-bit classical register that stores the results of qubit measurement. Moving from left to right in the diagram represents forward motion in time. Colored boxes on top of the qubit wires represent different quantum gates acting on their respective qubit. The blue box labeled  $H$  is the Hadamard gate; the green box labeled  $R_z$  is a rotation of the qubit about the  $z$ -axis by a given angle; blue two-qubit gates represented by circles with a cross are  $CNOT$  gates; and finally, magenta boxes represent measurements of qubits into the classical register.

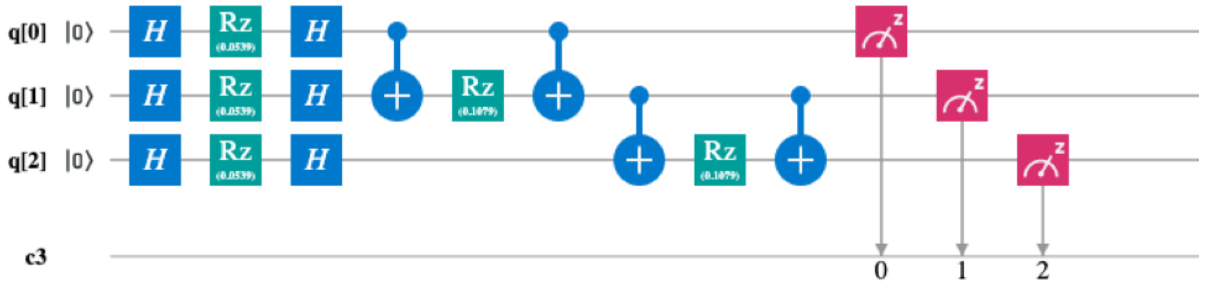

FIG. S3. Quantum circuit diagram simulating time evolution to the first time-step for a three-qubit system.

### Pseudocode for Dynamic Simulation on Quantum Computers

Table S1 shows pseudocode for a dynamic simulation of a quantum system for a total time  $T\Delta t$ . The full code is available in the included python notebooks.

TABLE SI. Pseudocode for dynamic simulation of qubits. For each simulated time-step, a different circuit is created. Next, in a user-define number of independent trials, the qubits are initialized to their  $t=0$  state, the particular circuit for the given time step is executed, and the qubits are measured. Measurements from all trial runs are averaged together to give an estimate for the final quantum state of the system at each time-step.

---

```

Set num_trials
For n in range(T):
    Create circuit  $C_n$  to simulate evolution to time step n with  $U(n\Delta t)$ 
    For i in range(num_trials):
        Initialize qubits to  $t=0$  state
        Run circuit  $C_n$ 

```

---

### Description of the Wavefunction Simulator

A wavefunction simulator uses a classical computer to simulate qubit evolution on a quantum computer by evaluating the many-body wavefunction of a system of  $N$  qubits (stored as a  $2^N \times 2^N$  matrix) after a set of gates (unitary matrices) has been applied to the initial wavefunction of the system. As such, unlike a real quantum computer, the wavefunction simulator provides access to the entire many-body quantum state (quantum computers only allow measurement of qubits, which collapses the full quantum state to a set of measured 0's and 1's). Furthermore, the wavefunction simulator does not experience any effects from noise or decoherence. Due to the exponential growth of the matrix storing the many-body wavefunction with the number of qubits in the system, wavefunction simulators cannot be efficiently used to simulate large systems. Results for small systems are nevertheless useful for validation purposes.

### Choice of the Time Discretization Unit

The simulated Hamiltonian is parameterized by three constants, namely  $J_z$ ,  $\varepsilon_{ph}$ ,  $\omega_{ph}$ , which each have associated frequencies. In order to find a suitable  $\Delta t$ , we must find the fastest frequency associated with the Hamiltonian and choose a  $\Delta t$  an order-of-magnitude smaller than one cycle of this frequency so as not to miss any dynamics. The frequency associated with  $J_z$  is  $J_z/h = 2.86265$  THz (where  $h$  is Planck's constant). The frequency associated with the largest  $\varepsilon_{ph}$  used in our simulations is  $(\varepsilon_{ph} = 5J_z)/h = 14.3133$  THz. Finally, the frequency associated with the phonon is  $f = \omega_{ph}/2\pi = 4.8$  THz. Thus, the highest frequency in our simulation Hamiltonian is 14.3133 THz, which has a period of 69.865 fs. We have chosen a time-step of 3 fs to adequately resolve this fast oscillation. As a validation, we ran our simulations with a time-step of 3 fs, 1.5 fs and 0.75 fs and obtained identical results.

### IBM's Q16 Melbourne Quantum Processor

One of the many currently available quantum computers from IBM, the Q16 Melbourne quantum processor has 14 qubits implemented with superconducting circuits. This quantum processor can natively perform three quantum gates on the qubits: (1) a two-qubit *CNOT* (or *CX*) gate, (2) a single-qubit *RX(theta)* gate, which performs a rotation of the qubit about the x-axis by

an angle  $\theta$  ( $\theta$  can only take on values of  $\pm \frac{\pi}{2}$ ), and (3) a single-qubit  $RZ(\theta)$  gate, which performs a rotation of the qubit about the  $z$ -axis by an angle  $\theta$  ( $\theta$  can take on any value in the range  $[0, 2\pi]$ ). Figure S4 shows the topology of the quantum processor.

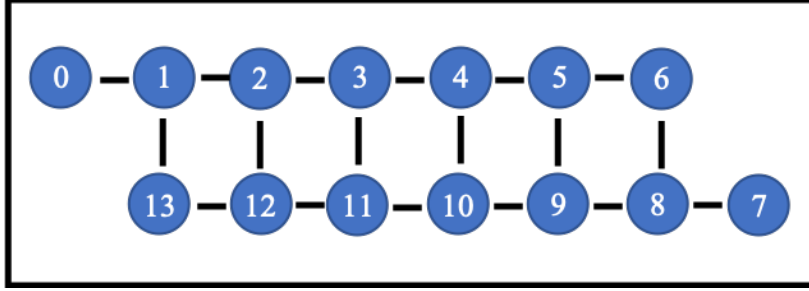

FIG. S4. Topology of the IBM Q16 Melbourne quantum processor. Blue circles represent qubits, while black lines represent physical connections between pairs of qubits.

The quantum processor can be accessed over the cloud with the use of IBM's python library Qiskit (see <https://qiskit.org/documentation/>). Quantum circuits for the processor can be developed using high-level functions provided by the Qiskit library. See the included python notebook 'QiskitDemo.ipynb' for more details on designing quantum circuits with Qiskit and connecting to the quantum processor.

Qubits 6 and 8 were used for all simulations. All simulations were run on September 28<sup>th</sup>, 2019. The decoherence and fidelity statistics for the quantum processor at the time of running were:

CNOT error rate between qubits 6 and 8: 3.695e-2  
 Qubit 6 T1: 59.385471279781605  
 Qubit 8 T1: 44.59902723438765  
 Qubit 6 T2: 77.58846374614568  
 Qubit 8 T2: 66.47979312575764  
 Qubit 6 Readout error: 3.5100000000000002e-2  
 Qubit 8 Readout error: 6.4100000000000005e-2  
 Qubit 6 single-qubit U3 error rate: 2.677611063734653e-3  
 Qubit 8 single-qubit U3 error rate: 5.813373587680526e-3

### Rigetti's Aspen Quantum Processor

The Rigetti Aspen quantum processor is comprised of 16 qubits implemented with superconducting qubits. The quantum processor can natively perform three gates on the qubits: (1) a two-qubit  $CZ$  gate, (2) a single-qubit  $RX(\theta)$  gate, which performs a rotation of the qubit about the  $x$ -axis by an angle  $\theta$  ( $\theta$  can only take on values of  $\pm\pi$  and  $\pm \frac{\pi}{2}$ ), and (3) a single-

qubit  $RZ(\theta)$  gate, which performs a rotation of the qubit about the  $z$ -axis by an angle  $\theta$  ( $\theta$  can take on any value in the range  $[0, 2\pi]$ ). Figure S5 shows the topology of the quantum processor.

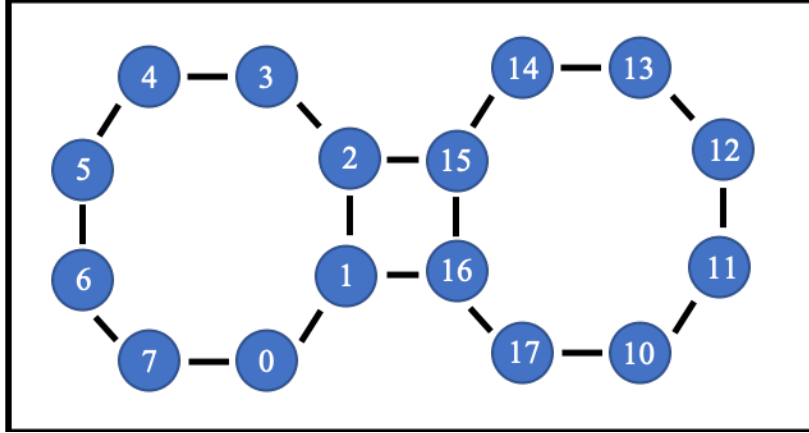

calculating the inner product of the many-body wavefunction and the average magnetization operator, the simulators simulate qubit measurement by stochastically collapsing each qubit to a 0 or a 1, according to their respective probabilities defined by the quantum state of the qubit. Therefore, simulating noisy qubits, like the quantum processor, requires averaging over many trials to approximate the quantum state of the system at each given time-step. Furthermore, both simulators allow for the user to set certain parameters to design their own noise model for the simulated qubits. The four main noise parameters that can be set are the decoherence times  $T1$  and  $T2$ ; the readout error, defined by  $p(0|0)$  (the probability that a qubit is read out as a ‘0’ given that it is in the ‘0’ state) and  $p(1|1)$  (the probability that a qubit is read out as a ‘1’ given that it is in the ‘1’ state); and on IBM’s simulator one can define the single-gate error rates. Readout errors are generally presumed to be symmetric, meaning the  $p(0|0) = p(1|1)$ . We set the noise parameters of our simulated noisy qubits to match those given for the qubits at the time of running our simulations on the quantum processors (given in the above sections about the quantum processors).

### **Simulation of Two-Dimensional Antiferromagnets**

While the main simulation results of this paper were performed for a system in the ferromagnetic initial state, our framework can easily be extended to the dynamic simulation of 2D antiferromagnets by initializing the qubits into the antiferromagnetic (AF) state. The AF state consists of nearest neighbor spins having opposite spin orientation. As both the IBM and Rigetti quantum computers initialize all qubits into the spin-up state, initializing the qubits in the AF state simply involves flipping every other qubit about the  $x$ -axis with the Pauli-X gate,  $\sigma_x$ . We performed dynamic simulations of the average magnetization for systems with 2-, 3-, 4-, and 5-qubits with the AF initial configuration. The systems were evolved under the Hamiltonian given in equation (1) in the main text, for different values of  $\varepsilon_{ph}$ . Results are summarized in Fig. S6, which show an even-odd parity effect, where varying the value of  $\varepsilon_{ph}$  has no discernable effect for systems with even numbers of qubits, but does for odd numbers of qubits.

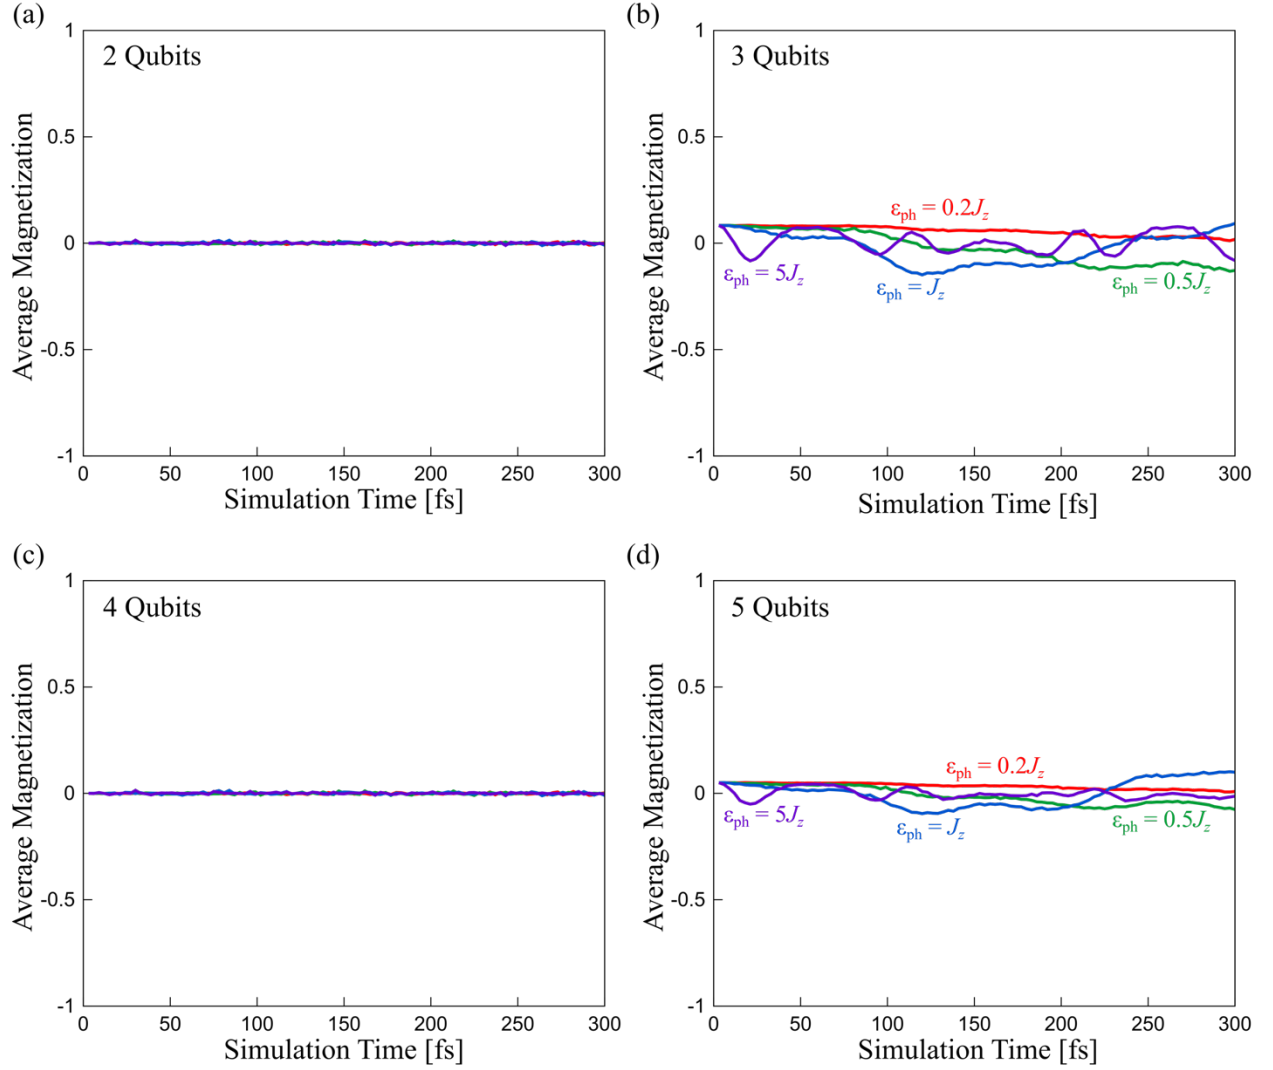

**FIG. S6.** Time evolution of the average magnetization of 2- (a), 3- (b), and 4- (c), and 5-qubit (d) systems that are initialized in the antiferromagnetic configuration. Results are shown for varying electron-phonon coupling strengths  $\epsilon_{ph} = 0.2J_z$  (red),  $0.5J_z$  (green),  $J_z$  (blue) and  $5J_z$  (purple).

## References for Supplemental Material

- [1] P. E. Blöchl, Phys. Rev. B **50**, 17953 (1994).
- [2] G. Kresse and D. Joubert, Phys. Rev. B **59**, 1758 (1999).
- [3] J. P. Perdew, K. Burke, and M. Ernzerhof, Phys. Rev. Lett. **77**, 3865 (1996).
- [4] A. I. Liechtenstein, V. I. Anisimov, and J. Zaanen, Phys. Rev. B **52**, R5467 (1995).
- [5] A. L. Ivanovskii, T. I. Chupakhina, V. G. Zubkov, A. P. Tyutyunnik, V. N. Krasilnikov, G. V. Bazuev, S. V. Okatov, and A. I. Lichtenstein, Phys. Lett. A **348**, 66 (2005).
- [6] S. Grimme, J. Comput. Chem. **27**, 1787 (2006).
- [7] F. Shimojo *et al.*, SoftwareX **10**, 100307 (2019).
- [8] F. Shimojo *et al.*, J. Chem. Phys. **140** (2014).
- [9] M. Kan, J. Zhou, Q. Sun, Y. Kawazoe, and P. Jena, J. of Phys. Chem. Lett. **4**, 3382 (2013).
- [10] A. Krishnamoorthy, L. Bassman, R. Kalia, A. Nakano, F. Shimojo, and P. Vashishta, Nanoscale **10**, 2742-2747 (2018).
- [11] D. Shin, H. Hübener, U. De Giovannini, H. Jin, A. Rubio, and N. Park, Natt Comm. **9**, 638 (2018).
- [12] G. Kresse and J. Furthmüller, Phys. Rev. B **54**, 11169 (1996).
